# Supplementary material for: Template-based Program Synthesis using Stellens\"atze
Source: arXiv:2209.03602 source file (2022-09-08)
Supplement: Supplementary file 1 [file appendix.tex]

\section{Appendix}
% \subsection{Proof of Theorems presented in Section \ref{synthesis_algo}}\label{appendix_proof}
% \begin{theorem}[Soundness, Proof in Appendix \ref{appendix_proof}]
% Given a polynomial program synthesis problem $(P,T,Q)$, the synthesis algorithm produces a valid program. More precisely the algorithm generates real valuation of template variables such that for all $\nu \in \mathbb{R}^V$, if $\nu \models P$ then $\mathbf{T}(\nu) \models Q$.
% \end{theorem}
% \begin{proof}

% \end{proof}

% \begin{theorem}[Semi-completeness, Proof in Appendix \ref{appendix_proof}]
% Let $(P,T,Q)$ be a polynomial program synthesis problem and $\mathbf{T}$ be any solution to the problem. Given sufficiently high values of technical constants $\{d_1,d_2,d_3,d_4)$, $\mathbf{T}$ can be realised using some solution of non-linear constraint system generated in \ref{algo_step_3} of our algorithm.
% \end{theorem}
% \begin{proof}

% \end{proof}

\subsection{Examples used in Section \ref{secion_proof_of_concept}}\label{appendix_examples}
These examples are motivated from the benchmarks provided in \cite{rodriguez2018some}.
